# Supplementary material for: Multi-class Token Transformer for Weakly Supervised Semantic Segmentation
Source: arXiv:2203.02891 source file (2022-03-06)
Supplement: Supplementary file 1 [file patch_aff.tex]

\begin{table}[t]
\caption{}
\vspace{-8pt}
\label{tab:patch_aff}
\small
\centering
\begin{tabular}{lccc}
\toprule 
          & 1  & 6 & 12                   \\ \midrule
mIoU &41.5&26.8&\textbf{47.2}\\
  \bottomrule 
\end{tabular}
% \end{center}
\vspace{-12pt}
\end{table}
