# Supplementary material for: Multi-class Token Transformer for Weakly Supervised Semantic Segmentation
Source: arXiv:2203.02891 source file (2022-03-06)
Supplement: Supplementary file 2 [file randwalk.tex]

% \begin{table}
% \centering
% \resizebox{\linewidth}{!}{ %< auto-adjusts font size to fill line
% \begin{tabular}{@{}lccc@{}}
% \toprule
% Method & Frobnability & Frobnability & Frobnability \\
% \midrule
% Ours v0 & Frumpy \\
% Ours v1 & Frobbly \\
% \textbf{Ours} & Makes one's heart Frob\\
% \bottomrule
% \end{tabular}
% } %< \resizebox
% \caption{
% % 
% \textbf{Ablations} -- our decisions are well justified.
% % 
% } % \caption
% \label{tab:ablations}
% \end{table}

\begin{table*}[t]
\caption{Segmentation results using the proposed pseudo labels before and after using random walk~\cite{ahn2018learning} in terms of mIoU (\%) on the PASCAL VOC \textit{val} set. $^{\star}$ denotes using post-processing on the segmentation results. }
\vspace{-8pt}
\label{tab:seed}
\small
\centering
\resizebox{\linewidth}{!}
{\begin{tabular}{lcccccccccccccccccccccc}
\toprule 
&bkg&plane&bike&bird&boat&bottle&bus&car&cat&chair&cow&table&dog&horse&mbk&person&plant&sheep&sofa&train&tv&mIoU \\
\midrule
\nn~& 87.8&56.5&34.5&72.2&43.3&67.8&76.5&76.3&83.1&26.9&69.0&50.5&78.2&68.6&69.2&65.1&49.3&72.1&44.6&68.6&54.8&62.6\\
\nn$^{\star}$&90.6&68.0&37.5&86.7&47.6&77.4&81.2&79.4&89.6&30.6&81.4&55.7&85.8&79.3&73.0&73.0&52.8&84.5&44.0&68.8&61.5&69.0 \\
 \midrule
 \multicolumn{23}{l}{With Random Walk~\cite{ahn2018learning}:} \\
\nn~& 90.6&71.8&37.5&85.1&52.9&68.8&78.8&78.7&87.1&28.4&78.9&53.0&83.9&78.2&76.8&76.4&54.1&80.1&46.0&71.6&54.3&68.2\\
\nn$^{\star}$&91.9&78.3&39.5&89.9&55.9&76.7&81.8&79.0&90.7&32.6&87.1&57.2&87.0&84.6&77.4&79.2&55.1&89.2&47.2&70.4&58.8&71.9 \\
  \bottomrule 
\end{tabular}
}
% \vspace{-18pt}
\end{table*}
